# Supplementary material for: Parsing Geometry Using Structure-Aware Shape Templates
Source: arXiv:1808.01337 source file (2018-09-05)
Supplement: Supplementary file 1 [file 20-appendix.tex]

%!TEX root = 00-main.tex
\section{Appendix}
\section{Supplementary Materials}
